# Supplementary material for: DEEMD: Drug Efficacy Estimation against SARS-CoV-2 based on cell Morphology with Deep multiple instance learning
Source: arXiv:2105.05758 source file (2022-06-16)
Supplement: Supplementary file 1 [file MIL_COVID_NC_Supp.pdf]

# Supplementary Material of DEEMD: Drug Efficacy Estimation against SARS-CoV-2 based on cell Morphology with Deep multiple instance learning

## 1 Noisy label analysis in MIL

As mentioned in subsection IV-B, the patch-based model  $\mathcal{V}(\psi)$  trains the model in the presence of noisy labels. To better understand this model and compare it to the MIL model  $\mathcal{M}(\theta)$ , it would be insightful to measure how much noise is in the training labels for both models. Each image is split into  $N$  patches and there are  $N_p$  positive samples and  $N_n$  negative samples in the dataset. We define the label noise in the dataset to be the ratio of the samples correctly labeled in the dataset to the total number of samples. Without loss of generality, assume that the fraction of the patches in a sample image that are truly infected has an expected value of  $\lambda$ . Therefore, the expected noise ratio (NR) for the MIL model  $\mathcal{M}(\theta)$  and the patch-based model  $\mathcal{V}(\psi)$  can be expressed as follows:

$$\text{NR}_{\mathcal{M}(\theta)} = \frac{|\frac{k}{N} - \lambda|N_p}{N_p + N_n}, \quad \text{NR}_{\mathcal{V}(\psi)} = \frac{(1 - \lambda)N_p}{N_p + N_n}. \quad (1)$$

By defining  $r(\lambda, \frac{k}{N})$  to be the log ratio of  $\text{NR}_{\mathcal{V}(\psi)}$  to  $\text{NR}_{\mathcal{M}(\theta)}$ , we can quantitatively analyze these two models behaviour in different configurations for  $\lambda$  and  $k$ .

$$r(\lambda, \frac{k}{N}) \triangleq \ln\left(\frac{\text{NR}_{\mathcal{V}(\psi)}}{\text{NR}_{\mathcal{M}(\theta)}}\right) = \ln\left(\frac{1 - \lambda}{|\frac{k}{N} - \lambda|}\right). \quad (2)$$

When  $r(\lambda, \frac{k}{N}) \geq 0$  the MIL model  $\mathcal{M}(\theta)$  has less noisy labels compared to the patch-based model  $\mathcal{V}(\psi)$ . The landscape of  $r(\lambda, \frac{k}{N})$  is visualized in Fig 1 for closer inspection. To ensure the numerical stability of  $r(\lambda, \frac{k}{N})$  and keep it bounded on the  $y = x$  line, a small value  $\epsilon$  was added to  $\text{NR}_{\mathcal{M}(\theta)}$ .

One can notice that in almost three forth of the cases,  $r(\lambda, \frac{k}{N}) \geq 0$ , meaning that the MIL model  $\mathcal{M}(\theta)$  has less noisy labels in its training procedure on average, hence, the model converges faster to an optimum point. Moreover, the MIL model  $\mathcal{M}(\theta)$  training procedure results in a more efficient training both in terms of computation footprint and extracted features. The model is using only  $k/N$  of the training set for updating the weights. This is  $N/k$  times faster than using the whole dataset in the patch-based model  $\mathcal{V}(\psi)$ . And more

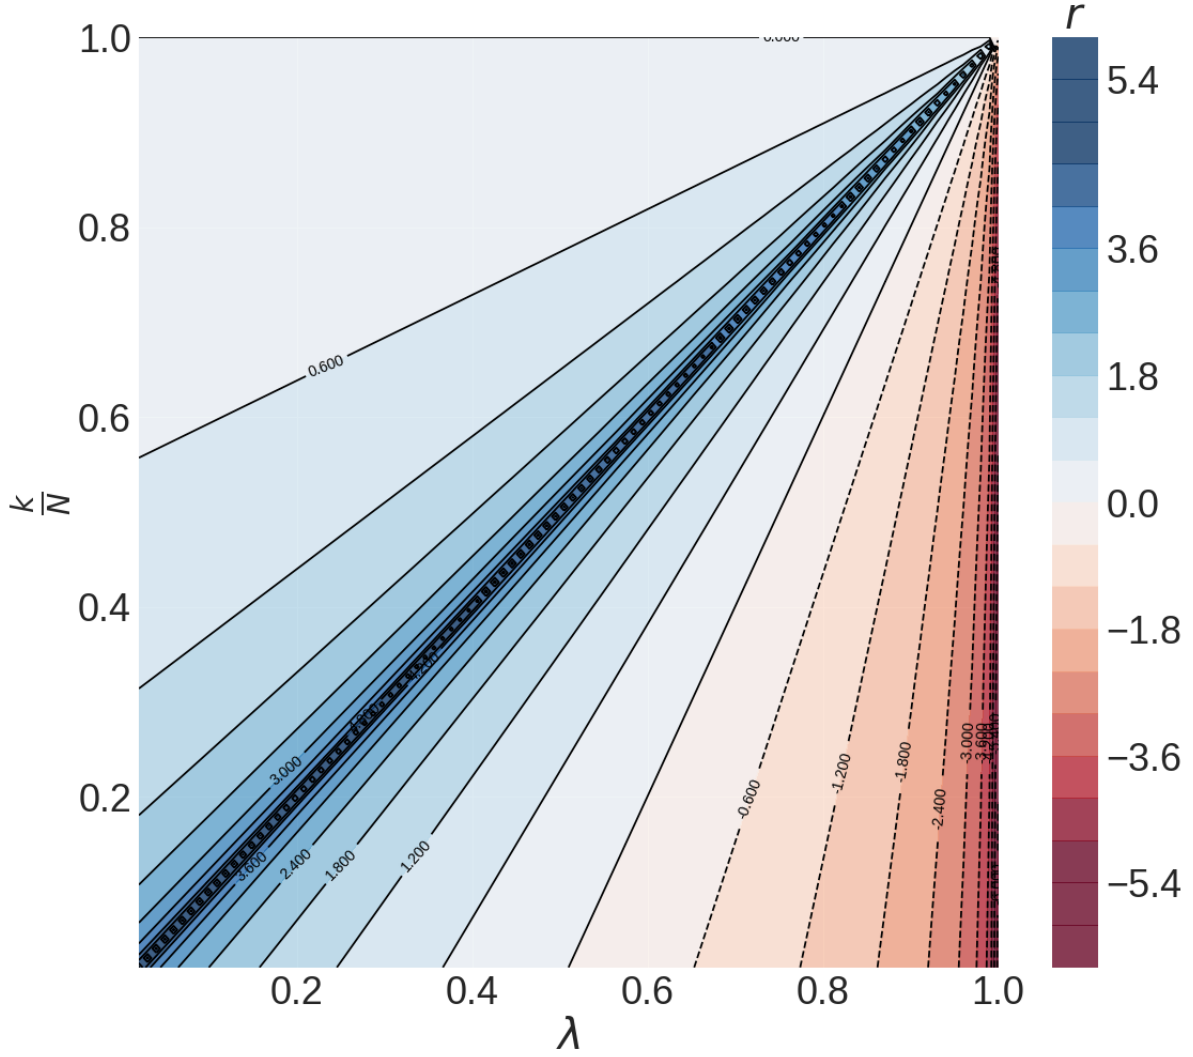

Figure 1: Contour plot for  $r(\lambda, \frac{k}{N})$ , all possible values for  $\lambda$  and  $\frac{k}{N}$  are shown on the x and y axis respectively.

importantly, the patches that are selected for training the MIL model  $\mathcal{M}(\theta)$ , would contain more discriminative features since they were top-ranked among all patches in their samples for their informativeness. Finally, the MIL model  $\mathcal{M}(\theta)$  has the capability of incorporating domain knowledge about the problem into the training by the choice of hyper-parameter  $k$ . By choosing  $k$  based on prior or domain knowledge, the MIL model  $\mathcal{M}(\theta)$  can iteratively refine its training dataset towards for less noisy labels.

| Rank | Compound          | Studies                               |
|------|-------------------|---------------------------------------|
| 1    | Remdesivir        | [4, 5, 12, 19, 20, 24, 31, 33, 35–37] |
| 2    | Digoxin           | [3, 31]                               |
| 3    | Aloxistatin       | [5, 12, 21, 22, 26, 36]               |
| 4    | Colchicine        | [6, 11, 25, 30, 36]                   |
| 5    | Mitoxantrone      | [38]                                  |
| 6    | Mebendazole       | [8, 18, 32]                           |
| 7    | Oxibendazole      | [18]                                  |
| 8    | GS-441524         | [19, 24, 27, 33, 35, 37]              |
| 9    | Thymoquinone      | [1, 7, 28, 34]                        |
| 10   | Lasalocid         | [29]                                  |
| 11   | Digitoxin         | [16, 17, 23]                          |
| 12   | Venetoclax        | [9]                                   |
| 13   | Homoharringtonine | [2, 4, 14, 15, 35, 36]                |
| 14   | Proscillaridin    | [10]                                  |
| 15   | Albendazole       | [18]                                  |
| 16   | Harringtonine     | -                                     |
| 17   | Gemcitabine       | [14, 35, 39]                          |
| 18   | Podophyllotoxin   | [13]                                  |

Table 1: Ranked list of DEEMD identified treatments,  $\mathcal{E}_{\mathcal{M}(\theta)}$ , along with drug repurposing or clinical studies that reported to show effectiveness against SARS-CoV-2 or COVID-19.

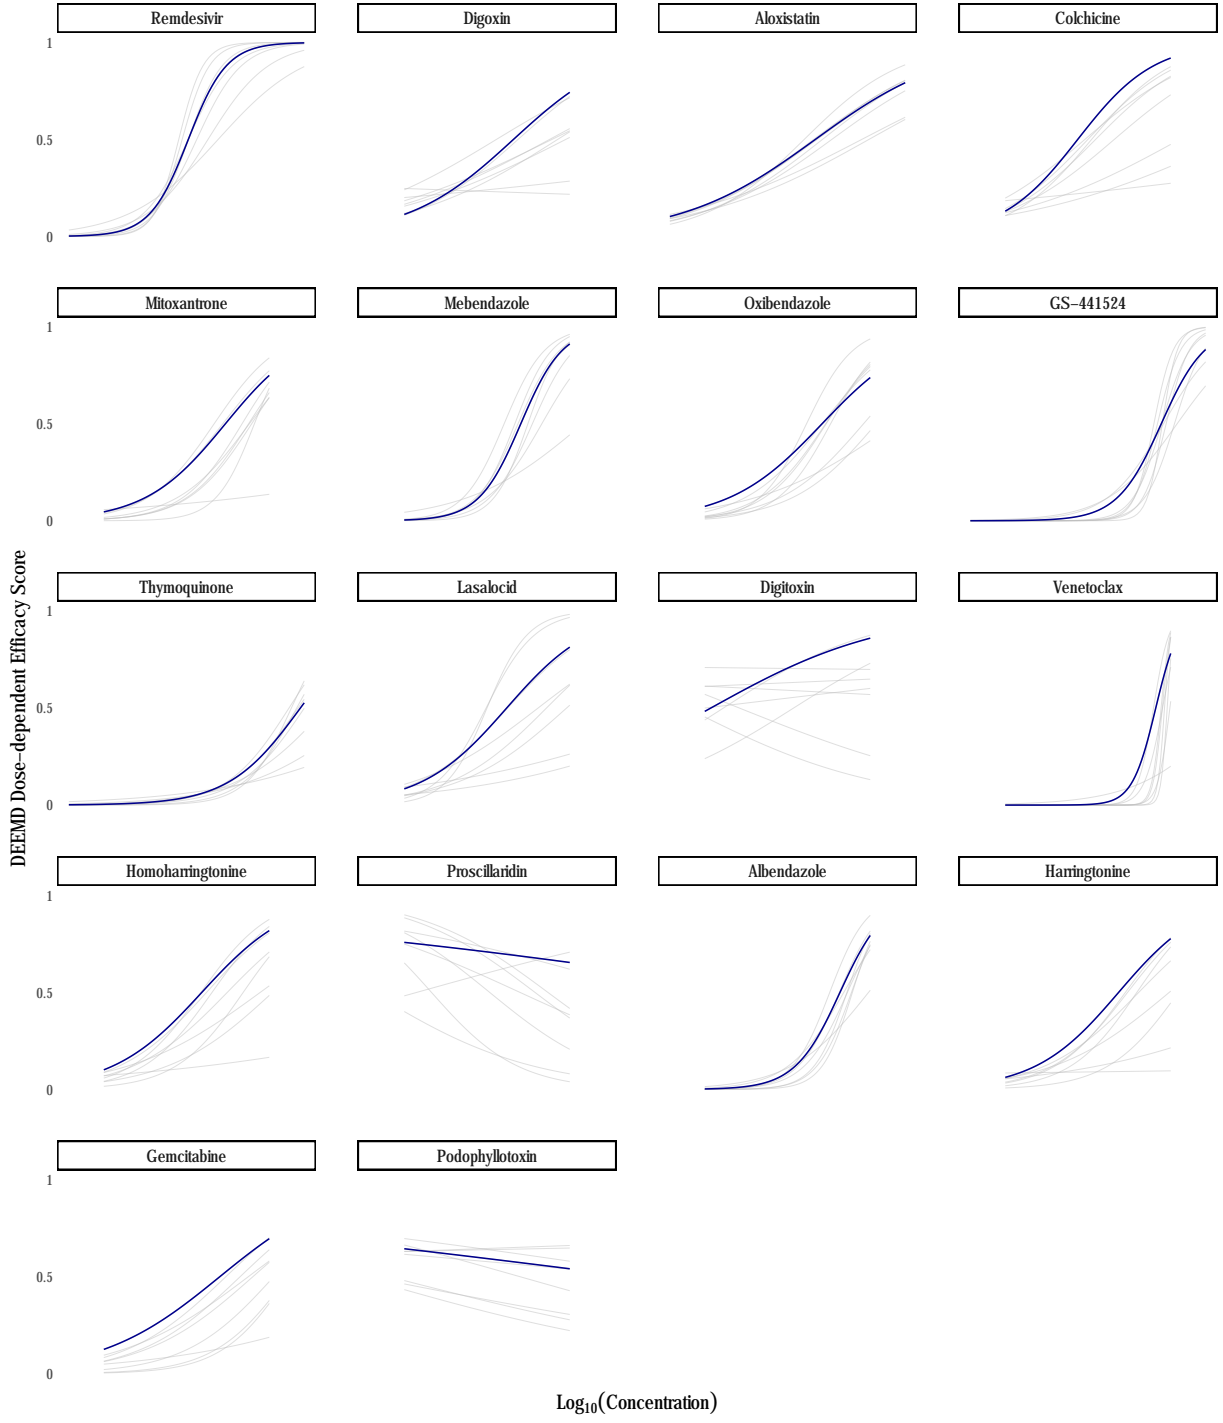

Figure 2: DEEMD estimated efficacy scores for identified treatments for different  $k$  values. The logistic curves are fitted based on each value for  $k$ . The blue curves represents the MIL model with  $k = 2$  which showed the best classification performance on the validation set.

## References

- [1] Ajaz Ahmad, Muneeb U Rehman, Parvaiz Ahmad, and Khalid M Alkharfy. Covid-19 and thymoquinone: Connecting the dots. *Phytotherapy Research*, 2020.
- [2] Yanwen Chen, Travis Lear, John Evankovich, Mads Larsen, Bo Lin, Irene Alfaras, Jason Kennerdell, Laura Salminen, Daniel Camarco, Karina Lockwood, et al. A high throughput screen for tmprss2 expression identifies fda-approved and clinically advanced compounds that can limit sars-cov-2 entry. 2020.
- [3] Junhyung Cho, Young Jae Lee, Je Hyoung Kim, Sang il Kim, Sung Soon Kim, Byeong-Sun Choi, and Jang-Hoon Choi. Antiviral activity of digoxin and ouabain against sars-cov-2 infection and its implication for covid-19. *Scientific reports*, 10(1):1–8, 2020.
- [4] Ka-Tim Choy, Alvina Yin-Lam Wong, Prathanporn Kaewpreedee, Sin-Fun Sia, Dong-dong Chen, Kenrie Pui Yan Hui, Daniel Ka Wing Chu, Michael Chi Wai Chan, Peter Pak-Hang Cheung, Xuhui Huang, et al. Remdesivir, lopinavir, emetine, and homoharringtonine inhibit sars-cov-2 replication in vitro. *Antiviral research*, page 104786, 2020.
- [5] Michael F Cuccarese, Berton A Earnshaw, Katie Heiser, Ben Fogelson, Chadwick T Davis, Peter F McLean, Hannah B Gordon, Kathleen-Rose Skelly, Fiona L Weathersby, Vlad Rodic, et al. Functional immune mapping with deep-learning enabled phenomics applied to immunomodulatory and covid-19 drug discovery. *bioRxiv*, 2020.
- [6] Medine Cumhuri Cure, Adem Kucuk, and Erkan Cure. Colchicine may not be effective in COVID-19 infection; it may even be harmful? *Clinical Rheumatology*, 39(7):2101–2102, May 2020.
- [7] Sawsan Elgohary, Aya A Elkhodiry, Nada S Amin, Ulrike Stein, and Hend M El Tayebi. Thymoquinone: a tie-breaker in sars-cov2-infected cancer patients? *Cells*, 10(2):302, 2021.
- [8] Ayman Farag, Ping Wang, Mahmoud Ahmed, and Hesham Sadek. Identification of fda approved drugs targeting covid-19 virus by structure-based drug repositioning. *ChemRxiv*, doi: doi, 10, 2020.
- [9] Moritz Fürstenau, Petra Langerbeins, Nisha De Silva, Anna Maria Fink, Sandra Robrecht, Julia von Tresckow, Florian Simon, Karin Hohloch, Jolanda Droogendijk, Marjolein van der Klift, et al. Covid-19 among fit patients with cll treated with venetoclax-based combinations. *Leukemia*, 34(8):2225–2229, 2020.
- [10] Kaifu Gao, Duc Duy Nguyen, Jiahui Chen, Rui Wang, and Guo-Wei Wei. Repositioning of 8565 existing drugs for covid-19. *arXiv preprint arXiv:2005.10028*, 2020.
- [11] Timotius Ivan Hariyanto, Devina Adella Halim, Claudia Jodhinata, Theo Audi Yanto, and Andree Kurniawan. Colchicine treatment can improve outcomes of coronavirus disease 2019 (covid-19): A systematic review and meta-analysis. *Clinical and Experimental Pharmacology and Physiology*, 2021.

- [12] Katie Heiser, Peter F McLean, Chadwick T Davis, Ben Fogelson, Hannah B Gordon, Pamela Jacobson, Brett L Hurst, Ben J Miller, Ronald W Alfa, Berton A Earnshaw, et al. Identification of potential treatments for covid-19 through artificial intelligence-enabled phenomic analysis of human cells infected with sars-cov-2. *bioRxiv*, 2020.
- [13] Andreas Hensel, Rudolf Bauer, Michael Heinrich, Verena Spiegler, Oliver Kayser, Georg Hempel, and Karin Kraft. Challenges at the time of covid-19: Opportunities and innovations in antivirals from nature. *Planta medica*, 86(10):659, 2020.
- [14] Aleksandr Ianevski, Rouan Yao, Svetlana Biza, Eva Zusinaite, Andres Mannik, Gaily Kivi, Anu Planken, Kristiina Kurg, Eva-Maria Tombak, Mart Ustav, et al. Identification of novel antiviral drug combinations in vitro and tracking their development. *bioRxiv*, 2020.
- [15] Aleksandr Ianevski, Rouan Yao, Mona Høysæter Fenstad, Svetlana Biza, Eva Zusinaite, Tuuli Reisberg, Hilde Lysvand, Kirsti Løseth, Veslemøy Malm Landsem, Janne Fossum Malmring, et al. Potential antiviral options against sars-cov-2 infection. *Viruses*, 12(6):642, 2020.
- [16] Sangeun Jeon, Meehyun Ko, Jihye Lee, Inhee Choi, Soo Young Byun, Soonju Park, David Shum, and Seungtaek Kim. Identification of antiviral drug candidates against sars-cov-2 from fda-approved drugs. *Antimicrobial Agents and Chemotherapy*, 2020.
- [17] Meehyun Ko, Sangeun Jeon, Wang-Shick Ryu, and Seungtaek Kim. Comparative analysis of antiviral efficacy of fda-approved drugs against sars-cov-2 in human lung cells. *Journal of medical virology*, 93(3):1403–1408, 2021.
- [18] Jeffrey N Law, Nure Tasnina, Meghana Kshirsagar, Judith Klein-Seetharaman, Mark Crovella, Padmavathy Rajagopalan, Simon Kasif, and TM Murali. Identifying human interactors of sars-cov-2 proteins and drug targets for covid-19 using network-based label propagation. *arXiv preprint arXiv:2006.01968*, 2020.
- [19] Yingjun Li, Liu Cao, Ge Li, Feng Cong, Yunfeng Li, Jing Sun, Yinzhu Luo, Guijiang Chen, Guanguan Li, Ping Wang, et al. Remdesivir metabolite gs-441524 effectively inhibits sars-cov-2 infection in mouse models. *Journal of medicinal chemistry*, 2021.
- [20] Carmen Mirabelli, Jesse W Wotring, Charles J Zhang, Sean M McCarty, Reid Fursmidt, Namrata S Kadambi, Anya T Amin, Teresa R O’Meara, Carla D Pretto-Kernahan, Jason R Spence, et al. Morphological cell profiling of sars-cov-2 infection identifies drug repurposing candidates for covid-19. *bioRxiv*, 2020.
- [21] Omonike A Olaleye, Manvir Kaur, Collins C Onyenaka, and Tolulope O Adebuseyi. Discovery of clioquinol and analogues as novel inhibitors of severe acute respiratory syndrome coronavirus 2 infection, ace2 and ace2-spike protein interaction in vitro. *bioRxiv*, 2020.
- [22] Xiuyuan Ou, Yan Liu, Xiaobo Lei, Pei Li, Dan Mi, Lili Ren, Li Guo, Ruixuan Guo, Ting Chen, Jiaxin Hu, et al. Characterization of spike glycoprotein of sars-cov-2 on

- virus entry and its immune cross-reactivity with sars-cov. *Nature communications*, 11(1):1–12, 2020.
- [23] Bette S Pollard, Jorge C Blanco, and John R Pollard. Classical drug digitoxin inhibits influenza cytokine storm, with implications for covid-19 therapy. *in vivo*, 34(6):3723–3730, 2020.
  - [24] Andrea J Pruijssers, Amelia S George, Alexandra Schäfer, Sarah R Leist, Lisa E Gralinski, Kenneth H Dinno III, Boyd L Yount, Maria L Agostini, Laura J Stevens, James D Chappell, et al. Remdesivir inhibits sars-cov-2 in human lung cells and chimeric sars-cov expressing the sars-cov-2 rna polymerase in mice. *Cell reports*, 32(3):107940, 2020.
  - [25] Naomi Schlesinger, Bonnie L Firestein, and Luigi Brunetti. Colchicine in covid-19: an old drug, new use. *Current Pharmacology Reports*, 6(4):137–145, 2020.
  - [26] Jian Shang, Yushun Wan, Chuming Luo, Gang Ye, Qibin Geng, Ashley Auerbach, and Fang Li. Cell entry mechanisms of sars-cov-2. *Proceedings of the National Academy of Sciences*, 117(21):11727–11734, 2020.
  - [27] Yuejun Shi, Lei Shuai, Zhiyuan Wen, Chong Wang, Yan Yuanyuan, Zhe Jiao, Fenglin Guo, Zhen F Fu, Chen Huanchun, Zhigao Bu, et al. The preclinical inhibitor gs441524 in combination with gc376 efficaciously inhibited the proliferation of sars-cov-2 in the mouse respiratory tract. *Emerging Microbes & Infections*, pages 1–43, 2021.
  - [28] Andrei P Sommer, Horst-Dieter Försterling, and Kurt G Naber. Thymoquinone: shield and sword against sars-cov-2. *Precis Nanomed*, 3(3):541–548, 2020.
  - [29] Esben B Svenningsen, Jacob Thyrsted, Julia Blay-Cadanet, Han Liu, Shaoquan Lin, Jaime Moyano-Villameriel, David Oलगnier, Manja Idorn, Søren R Paludan, Christian K Holm, et al. Ionophore antibiotic x-206 is a potent inhibitor of sars-cov-2 infection in vitro. *Antiviral research*, 185:104988, 2021.
  - [30] Jean-Claude Tardif, Nadia Bouabdallaoui, Philippe L L’Allier, Daniel Gaudet, Binita Shah, Michael H Pillinger, Jose Lopez-Sendon, Protasio da Luz, Lucie Verret, Sylvia Audet, et al. Efficacy of colchicine in non-hospitalized patients with covid-19. *Medrxiv*, 2021.
  - [31] Philip L Tzou, Kaiming Tao, Janin Nouhin, Soo-Yon Rhee, Benjamin D Hu, Shruti Pai, Neil Parkin, and Robert W Shafer. Coronavirus antiviral research database (cov-rdb): an online database designed to facilitate comparisons between candidate anti-coronavirus compounds. *Viruses*, 12(9):1006, 2020.
  - [32] Zhihan Wang, Kai Guo, Pan Gao, Qinqin Pu, Min Wu, Changlong Li, and Junguk Hur. Identification of repurposable drugs and adverse drug reactions for various courses of covid-19 based on single-cell rna sequencing data. *ArXiv*, 2020.

- [33] Xuping Xie, Antonio E Muruato, Xianwen Zhang, Kumari G Lokugamage, Camila R Fontes-Garfias, Jing Zou, Jianying Liu, Ping Ren, Mini Balakrishnan, Tomas Cihlar, et al. A nanoluciferase sars-cov-2 for rapid neutralization testing and screening of anti-infective drugs for covid-19. *Nature communications*, 11(1):1–11, 2020.
- [34] Huan Xu, Bing Liu, Zhen Xiao, Meiling Zhou, Lin Ge, Fan Jia, Yanling Liu, Hongshan Jin, Xiuliang Zhu, Jian Gao, et al. Computational and experimental studies reveal that thymoquinone blocks the entry of coronaviruses into in vitro cells. *Infectious diseases and therapy*, pages 1–12, 2021.
- [35] Cheng-Wei Yang, Tzu-Ting Peng, Hsing-Yu Hsu, Yue-Zhi Lee, Szu-Huei Wu, Wen-Hsing Lin, Yi-Yu Ke, Tsu-An Hsu, Teng-Kuang Yeh, Wen-Zheng Huang, et al. Repurposing old drugs as antiviral agents for coronaviruses. *Biomedical journal*, 43(4):368–374, 2020.
- [36] Hassan Yousefi, Ladan Mashouri, Samuel C Okpechi, Nikhilesh Alahari, and Suresh K Alahari. Repurposing existing drugs for the treatment of covid-19/sars-cov-2 infection: A review describing drug mechanisms of action. *Biochemical pharmacology*, page 114296, 2020.
- [37] Keivan Zandi, Franck Amblard, Katie Musall, Jessica Downs-Bowen, Ruby Kleinbard, Adrian Oo, Dongdong Cao, Bo Liang, Olivia O Russell, Tamara McBrayer, et al. Repurposing nucleoside analogs for human coronaviruses. *Antimicrobial Agents and Chemotherapy*, 65(1), 2020.
- [38] Qi Zhang, Catherine Zhengzheng Chen, Manju Swaroop, Miao Xu, Lihui Wang, Juhyung Lee, Amy Qiu Wang, Manisha Pradhan, Natalie Hagen, Lu Chen, Min Shen, Zhiji Luo, Xin Xu, Yue Xu, Wenwei Huang, Wei Zheng, and Yihong Ye. Heparan sulfate assists SARS-CoV-2 in cell entry and can be targeted by approved drugs in vitro. *Cell Discovery*, 6(1), November 2020.
- [39] Ya-Nan Zhang, Qiu-Yan Zhang, Xiao-Dan Li, Jin Xiong, Shu-Qi Xiao, Zhen Wang, Zhe-Rui Zhang, Cheng-Lin Deng, Xing-Lou Yang, Hong-Ping Wei, et al. Gemcitabine, lycorine and oxysophoridine inhibit novel coronavirus (sars-cov-2) in cell culture. *Emerging microbes & infections*, 9(1):1170–1173, 2020.
